# Supplementary material for: Multi-Frame GAN: Image Enhancement for Stereo Visual Odometry in Low Light
Source: arXiv:1910.06632 source file (2019-10-15)
Supplement: Supplementary file 1 [file appendix.tex]

% !TeX root = ../suppl.tex

\section{Introduction}
In this supplementary material, we firstly show the details of the network 
architecture of MFGAN. Then, we introduce more information regarding how 
Oxford RobotCar dataset~\cite{maddern20171} is used to evaluate our method and 
present the qualitative results of flow estimation on different light 
environment.
Next, we show the 
experiments of New Tsukuba dataset~\cite{martull2012realistic} and additional 
results on Oxford RobotCar dataset. Additionally, we also provide a 
supplementary video 
to demonstrate the performance of MFGAN for the frame consistency as well as 
the improvement for stereo VO methods.

\section{Network Details}

The detailed architecture for the encoder and decoder of the generators is 
shown in Figure~\ref{fig:Gencoder} and Figure~\ref{fig:Gdecoder}, respectively. 
We extend the architecture of \cite{zhu2017unpaired} to take into account 
temporal consistency and 
stereo image pairs. During training, the networks share the 
weights in Siamese networks fashion \cite{koch2015siamese} to push consistency over frames and 
optimize the parameters all together after forwarding two temporally neighboring stereo pairs. Note 
that we do not separately train the networks for optical flow estimation but 
use the supervision of the estimated optical flow only in the training phase.

\begin{figure}
	\begin{minipage}[b]{0.5\linewidth}
		\centering
		\includegraphics[width=\textwidth]{./figures/Gencoder.png}
		\caption{Encoder architecture of the generator network. 
		The encoder takes the concatenated stereo image pair 
		at the same timestamp and generates the corresponding feature. 
		The convolutional layers are shown with the kernel size and 
		the number of output channels followed by 9 residual blocks.}
		\label{fig:Gencoder}
	\end{minipage}
	\hspace{0.5cm}
	\begin{minipage}[b]{0.5\linewidth}
		\centering
		\includegraphics[width=\textwidth]{./figures/Gdecoder.png}
		\caption{Decoder architecture of the generator network. We generate the features from two 
		consecutive temporal stereo pairs and concatenate the features to feed into 
		the decoder part. Transposed convolutional layers for upsampling are presented in yellow color.} 
		\label{fig:Gdecoder}
	\end{minipage}
\end{figure}

\begin{figure}[h]
	\centering
	\includegraphics[width=0.8\linewidth,]{./figures/oxfordroute_small.jpg}
	\caption{The entire route of the Oxford RobotCar dataset (left image) is represented in green route 
		and 10 sub-sequences taken from the whole trajectory (right image) are marked in yellow color 
		respectively.} \label{fig:oxford_subseqs}
\end{figure}

\section{Details of using Oxford RobotCar Dataset}

The Oxford RobotCar dataset \cite{maddern20171} contains a large amount of data collected while 
traversing approximately 10km in central Oxford, UK for a year in different time slots and weathers. We 
divide the entire sequence into 10 sub-sequences where each sequence is around 700m distance and 
has certain characteristics of the trajectories. These sub-sequences are shown 
on Oxford map in Figure \ref{fig:oxford_subseqs}. Most of sequences contain one or more 
curves, Seq. 3 has difficult U-turn route, and Seq. 6 is straight-shaped road. 
For training, we split the sequences such that they are equally distributed 
on the entire map. We use Seq. 0, 2, 3, 5, 8 as training set and 
Seq. 1, 4, 6, 7, 9 as testing sequences. Note that there are no overlaps 
between the training set and the test.

We take the same sequences from different conditions using GPS/INS data from the Oxford RobotCar 
dataset. First, we fix the start point of each sequence according to GPS location from Day set and take 
the corresponding sequence from Night set using the fixed GPS position. Then, we set the end of each 
sequence by measuring the same distance. To generate ground-truth poses for the evaluation of VO 
methods, since the timestamps of frames are not synchronized with GPS/INS data, we interpolated the 
pose of timestamps based on GPS/INS data. 
In addition, we cut the car head part fixed at the bottom in the 
frames because the fixed objects unrelated with the scene cause difficulties to run VO methods.

\clearpage

\section{Flow Estimation on Different Lighting Images}
We check that FlowNet2 in general shows good performance 
for not only bright lighting but also dark illumination images. The predicted optical flow on Day 
and Night scene of the Oxford RobotCar dataset is shown in Figure \ref{fig:flowestimation} 
with a warped image based on the flow. Additionally, the evaluation results on the main paper 
show that, with the estimation quality delivered by FlowNet2, MFGAN is able to generate 
temporal as well as stereo consistent sequences.

\begin{figure}[h]
	\centering
	\includegraphics[width=1.0\linewidth,]{./figures/flowestimation.jpg}
	\caption{Flow estimation and warped images of Day and Night scene in the Oxford
RobotCar dataset. The first row is made of images of Day set and the second
row consists of images from Night set. The estimated flows show the fair 
quality of warped images leading to reasonable supervision for consistency.} \label{fig:flowestimation}
\end{figure}

\section{More Experiments}

\subsection{New Tsukuba Dataset}

This synthetic dataset \cite{martull2012realistic} captures static office scene. The dataset contains 
1800 stereo image pairs with ground-truth camera pose, disparity maps, occlusion maps and 
discontinuity maps. The stereo camera travels the fixed trajectory under different lighting such as 
Daylight, Fluorescent, Lamps and Flashlight, and the camera poses demonstrate strong 
rotation change. We test our method on one pair of unpaired sets, 
\textit{Fluorescent} and \textit{Flashlight}, and used 1000 images as a training set 
and 800 images for the evaluation. Although the images in \textit{Fluorescent} and 
\textit{Flashlight} set are paired, we utilize them in unpaired setting when training.

The experiments about frame consistency and VO performance on test sequences are shown in Table 
\ref{tab:epe_temporal_tsukuba} and \ref{tab:tsukuba_eval}, respectively. 
The enhanced sequence by the model $cy,tmp$ trained with temporal consistency as 
well as cycle consistency shows better frame consistency and improves the VO performance of both
direct and indirect methods compared to when using original \textit{Flashlight} and the $cy$ outputs.
Further adding the stereo consistency did not improve the results on this 
dataset.

\begin{table}[h]
	\centering
	\scriptsize
	\begin{tabular}{c|c|c}
		\hline
		& $cy$ &  $cy,tmp$ \\
		\hline
		median  & 0.75 & \textbf{0.54} 
		\\
		mean  & 2.20 & \textbf{1.68}
		\\
		\hline
	\end{tabular}
	\caption{EPE $E_{tmp}$ of the New Tsukuba dataset for temporal 
		consistency.}
	\label{tab:epe_temporal_tsukuba}
\end{table}

\begin{table*}[h]
	\centering
	\scriptsize
	\begin{tabular}{c|cc||cc|cc}
		\hline
		& \multicolumn{2}{c||}{Flashlight} & 
		\multicolumn{2}{c|}{$cy$} & 
		\multicolumn{2}{c}{$cy,tmp$}\\ 
		& $t_{abs}$ & $r_{abs}$ & $t_{abs}$ & $r_{abs}$ 
		& $t_{abs}$ & $r_{abs}$
		\\
		\hline
		DSO  & 2.055 & 39.35 & 0.194 & 2.34 & \textbf{0.144} & 
		\textbf{2.06}
		\\
		ORB  & X & X &  0.284 & 8.63 & \textbf{0.239} & 
		\textbf{7.86}
		\\
		\hline
	\end{tabular}
	\caption{Evaluation on the New Tsukuba dataset. $t_{abs}(m)$ and 
		$t_{abs}(^\circ)$ are absolute translation and rotational RMSE. The 
		image 
		translation model $cy$ allows stereo VO methods outperform on dark 
		scene, 
		and adding temporal consistency $cy,tmp$ leads to even better 
		performance.} 
	\label{tab:tsukuba_eval}
\end{table*}

Note that we measure the absolute trajectory error because the test sequence 
is short, i.e., less than 50m.

%\begin{table*}[h]
%	\centering
%	\scriptsize
%	\begin{tabular}{c|cc||cc|cc|cc}
%		\hline
%		& \multicolumn{2}{c||}{Fluorescent} & 
%		\multicolumn{2}{c|}{Flashlight} & 
%		\multicolumn{2}{c|}{$cy$} 
%		& 
%		\multicolumn{2}{c}{$cy,tmp$}\\ 
%		& $t_{abs}$ & $r_{abs}$ & $t_{abs}$ & $r_{abs}$ & $t_{abs}$ & $r_{abs}$ 
%		& $t_{abs}$ & $r_{abs}$
%		\\
%		\hline
%		DSO  & 0.092 & 1.30 & 2.055 & 39.35 & 0.194 & 2.34 & \textbf{0.144} & 
%		\textbf{2.06}
%		\\
%		ORB  & 0.177 & 5.61 & X & X &  0.284 & 8.63 & \textbf{0.239} & 
%		\textbf{7.86}
%		\\
%		\hline
%	\end{tabular}
%	\caption{Evaluation on the New Tsukuba dataset. $t_{abs}(m)$ and 
%		$t_{abs}(^\circ)$ are absolute translation and rotational RMSE.The 
%		image 
%		translation model $cy$ allows stereo VO methods outperform on dark 
%		scene, 
%		and adding temporal consistency $cy,tmp$ leads to even better 
%		performance.} 
%	\label{tab:tsukuba_eval}
%\end{table*}

\subsection{Oxford RobotCar Dataset}

The estimated trajectories of Seq. 1, 6, 7 by Stereo DSO are shown 
in the left side of Figure \ref{fig:traj01}, \ref{fig:traj06} and \ref{fig:traj07}, and 
those by stereo ORB-SLAM are shown in the right side of the figures.

\begin{figure*}[h]
	\includegraphics[width=.5\textwidth]{./figures/ablation_traj/plot_dso_01_0.png}
	\includegraphics[width=.5\textwidth]{./figures/ablation_traj/plot_orb_01_0.png}
	\caption{Seq. 1 of Oxford RobotCar dataset from Stereo DSO (left) 
	and stereo ORB-SLAM 
	(right).}
	\label{fig:traj01}
\end{figure*}

\begin{figure*}[h]
	\includegraphics[width=.5\textwidth]{./figures/ablation_traj/plot_dso_06_1.png}
	\includegraphics[width=.5\textwidth]{./figures/ablation_traj/plot_orb_06_3.png}
	\caption{Seq. 6 of Oxford RobotCar dataset from Stereo DSO (left) 
		and stereo ORB-SLAM 
		(right).}
	\label{fig:traj06}
\end{figure*}

\begin{figure*}[h]
	\includegraphics[width=.5\textwidth]{./figures/ablation_traj/plot_dso_07_2.png}
	\includegraphics[width=.5\textwidth]{./figures/ablation_traj/plot_orb_07_3.png}
	\caption{Seq. 7 of Oxford RobotCar dataset from Stereo DSO (left) 
		and stereo ORB-SLAM 
		(right).}
	\label{fig:traj07}
\end{figure*}

\subsection{Stereo Visual Odometry with Different Lighting}

We evaluate the VO performance using both direct and indirect methods 
on different lighting conditions, i.e., a bright optimal scene and a dark challenging scene without any 
image enhancement. 

With New Tsukuba dataset, the results on Fluorescent and Flashlight are 
shown in Table \ref{tab:tsukuba_naive_eval}. It is clearly observed that 
 that Stereo DSO and stereo ORB-SLAM on Fluorescent scene deliver
 accurate as well as robust performance compared to on Flashlight scene 
 e.g., losing tracking.
 
 \begin{table*}[h]
 	\centering
 	\scriptsize
 	\begin{tabular}{c|cc|cc}
 		\hline
 		& \multicolumn{2}{c|}{Fluorescent} & 
 		\multicolumn{2}{c}{Flashlight}\\ 
 		& $t_{abs}$ & $r_{abs}$ & $t_{abs}$ & $r_{abs}$	\\
 		\hline
 		DSO  & \textbf{0.092} & \textbf{1.30} & 2.055 & 39.35	\\
 		ORB  & \textbf{0.177} & \textbf{5.61} & X & X\\
 		\hline
 	\end{tabular}
 	\caption{Evaluation on the New Tsukuba dataset. X indicates the 
 		tracking is lost.} 
 	\label{tab:tsukuba_naive_eval}
 \end{table*}
 
 With Oxford RobotCat dataset, we evaluate the test sequences of a Day set, 
 and the results are shown in Table \ref{tab:oxford_naive_result} with the 
 results on Night scene. As proposed in the KITTI Odometry 
 Benchmark~\cite{geiger2012we}, we evaluate 
 the relative translational error ($t_{rel}$) and relative rotational 
 error ($r_{rel}$) as a function of trajectory length. Specifically, the 
 metrics 
 are defined as
 
 \begin{equation}
 t_{rel}(\mathcal{F}) = 
 \frac{1}{|\mathcal{F}|}\sum_{(i,j)\in\mathcal{F}}||(\mathbf{\hat{p}}_j \ominus 
 \mathbf{\hat{p}}_i) \ominus (\mathbf{p}_j \ominus \mathbf{p}_i)||_2
 \end{equation}
 \begin{equation}
 r_{rel}(\mathcal{F}) = 
 \frac{1}{|\mathcal{F}|}\sum_{(i,j)\in\mathcal{F}}\angle[(\mathbf{\hat{p}}_j 
 \ominus 
 \mathbf{\hat{p}}_i) \ominus (\mathbf{p}_j \ominus \mathbf{p}_i)]
 \end{equation}
 where $\mathcal{F}$ is a set of frames $(i,j)$, $\mathbf{\hat{p}} \in SE(3)$ 
 and $\mathbf{p} \in SE(3)$ are estimated and true camera poses, respectively, 
 $\ominus$ denotes the inverse compositional operator and $\angle[\cdot]$ is 
 the rotation angle.  
 
 The results show that a Day scene with bright illumination gives more accurate 
 and reliable performance of stereo VO methods than a Night scene.
 
 \begin{table*}[h]
 	\centering
 	\scriptsize
 	\begin{tabular}{cc|cc|cc}
 		\hline
 		& & \multicolumn{2}{c|}{Day} &
 		\multicolumn{2}{c}{Night}\\ 
 		Seq. & & $t_{rel}$ & $r_{rel}$ & $t_{rel}$ & 
 		$r_{rel}$\\
 		\hline
 		\multirow{2}{*}{01}  
 		& DSO & 7.86 & \textbf{1.71} & \textbf{7.16} & 2.91\\
 		& ORB & \textbf{7.16} & \textbf{2.10} & X & 4.80\\
 		\hline
 		\multirow{2}{*}{04}
 		& DSO & \textbf{7.13} & \textbf{2.01} & 24.78 & 5.28\\
 		& ORB & \textbf{3.78} & \textbf{1.90} & X & 11.00\\
 		\hline
 		\multirow{2}{*}{06}
 		& DSO & \textbf{9.07} & \textbf{0.71} & 9.86 & 0.87\\
 		& ORB & 5.73 & \textbf{0.61} & \textbf{5.52} & 0.86\\
 		\hline
 		\multirow{2}{*}{07}
 		& DSO & \textbf{6.07} & \textbf{1.79} & 6.38 & 2.38\\
 		& ORB & \textbf{3.52} & \textbf{2.26} & 6.35 & 2.58\\
 		\hline
 		\multirow{2}{*}{09}
 		& DSO & \textbf{5.32} & \textbf{2.07} & 7.87 & 4.96\\
 		& ORB & \textbf{4.27} & \textbf{2.20} & 14.16 & 9.21\\
 		\hline
 		\hline
 		\multirow{2}{*}{mean}
 		& DSO & \textbf{7.09} & \textbf{1.80} & 11.21 & 3.28\\
 		& ORB & \textbf{4.89} & \textbf{1.81} & 16.94 & 5.69\\
 		\hline
 	\end{tabular}
 	\caption{Comparison of Day and Night sequences of Oxford RobotCar dataset. 
 		$t_{rel}(\%)$ and $r_{rel}(^\circ)$ are the relative translational and 
 		rotational errors~\cite{geigerwe}. Note that although the corresponding 
 		Day and Night sequences share similar trajectories, there are no 1-to-1 
 		paired images. Overall, both VO systems deliver more accurate results 
 		on Day sequences. For the sequences where Night is better than Day, our 
 		observation is that these Night sequences are with fairly good lighting 
 		conditions and contain less dynamic objects than the corresponding Day 
 		sequences.}
 	\label{tab:oxford_naive_result}
 \end{table*}
 
 \subsection{Qualitative Results of Other Methods}
 
 In the paper, we compare MFGAN with other methods to evaluate 
 VO performance. The example frames of Oxford RobotCar dataset 
 generated by other methods are shown in Figure \ref{fig:benchmark}.
 We tested the enhanced sequence by photo enhancement methods: 
 adaptive histogram equalization(AHE)~\cite{zuiderveld1994contrast}, low-light image 
 enhancement(LIME)~\cite{guo2016lime}, and deep photo 
 enhancer(DP)~\cite{deephotoenhancer}. The frames translated by 
 style transfer methods such as ToDayGAN~\cite{anoosheh2018night}, DRIT~\cite{DRIT}, and 
 LinearTransfer(LT)~\cite{li2018learning} are presented as well.

\begin{figure}
	\centering
	\begin{subfigure}{\linewidth}
		\includegraphics[width=\linewidth]{./figures/benchmark1_small.jpg}
		\caption{} 
	\end{subfigure}
\par\bigskip
	\begin{subfigure}{\linewidth}
		\includegraphics[width=\linewidth]{./figures/benchmark2_small.jpg}
		\caption{}
	\end{subfigure}
	\caption{Enhanced frame examples. The top left image is the original 
		Night image and the other images in the first row are generated from 
		photo enhancement methods. On the second row, the first three images 
		are translated by other style transfer methods, and the last image is 
		by MFGAN.}
	\label{fig:benchmark}
\end{figure}
